# Supplementary material for: Combining Renormalized Singles $GW$ Methods with the Bethe-Salpeter Equation for Accurate Neutral Excitation Energies
Source: arXiv:2206.15034 ancillary file (2022-10-17)
Supplement: Supplementary file 1 [file bse_rsgw_manuscript.pdf]

# Supporting Information: Combining Renormalized Singles $GW$ Methods with the Bethe-Salpeter Equation for Accurate Neutral Excitation Energies

Jiachen Li,[†] Dorothea Golze,[‡] and Weitao Yang[*,†]

†*Department of Chemistry, Duke University, Durham, NC 27708, USA*

‡*Faculty of Chemistry and Food Chemistry, Technische Universität Dresden, 01062 Dresden, Germany*

E-mail: weitao.yang@duke.edu

## 1 Fundamental gaps obtained from $G_0W_0$, $G_{\mathbf{RS}}W_0$, $G_{\mathbf{RS}}W_{\mathbf{RS}}$ and ev$GW$

Table S1: Fundamental gaps of molecules in Truhlar-Gagliardi test set[S1] obtained from $G_0W_0$, $G_{\mathrm{RS}}W_0$, $G_{\mathrm{RS}}W_{\mathrm{RS}}$ and ev$GW$ based on BLYP. The aug-cc-pVDZ basis set was used for naphthalene, pNA and DMABN, and the aug-cc-pVTZ basis set was used for the remaining systems. B-TCNE was not included because of computational cost. All values in eV.

| | $G_0W_0$@BLYP | $G_{\mathrm{RS}}W_0$@BLYP | $G_{\mathrm{RS}}W_{\mathrm{RS}}$@BLYP | ev$GW$@BLYP |
|---|---|---|---|---|
| acetaldehyde | 10.80 | 11.75 | 12.47 | 12.25 |
| acetone | 10.40 | 11.31 | 12.06 | 11.78 |
| formaldehyde | 11.30 | 12.17 | 12.81 | 12.63 |
| pyrazine | 8.98 | 9.69 | 10.29 | 10.12 |
| pyridazine | 8.46 | 9.31 | 9.94 | 9.73 |

Table S1: Continued

| | $G_0W_0$@BLYP | $G_{\mathrm{RS}}W_0$@BLYP | $G_{\mathrm{RS}}W_{\mathrm{RS}}$@BLYP | ev$GW$@BLYP |
|---|---|---|---|---|
| pyridine | 9.59 | 10.30 | 10.94 | 10.79 |
| pyrimidine | 9.33 | 10.06 | 10.70 | 10.53 |
| s-tetrazine | 7.61 | 8.36 | 8.99 | 8.81 |
| ethylene | 12.16 | 12.54 | 13.00 | 12.92 |
| butadiene | 9.47 | 9.85 | 10.29 | 10.20 |
| benzene | 10.14 | 10.56 | 10.99 | 10.86 |
| naphthalene | 7.88 | 8.27 | 8.67 | 8.58 |
| furan | 10.42 | 10.79 | 11.23 | 11.12 |
| hexatriene | 7.89 | 8.28 | 8.70 | 8.62 |
| water | 12.81 | 13.69 | 14.19 | 13.99 |
| pNA | 7.27 | 7.87 | 8.42 | 8.30 |
| DMABN | 7.90 | 8.37 | 8.85 | 8.74 |

Table S2: Fundamental gaps of molecules in Truhlar-Gagliardi test set[S1] obtained from $G_0W_0$, $G_{\mathrm{RS}}W_0$, $G_{\mathrm{RS}}W_{\mathrm{RS}}$ and ev$GW$ based on PBE. The aug-cc-pVDZ basis set was used for naphthalene, pNA and DMABN, and the aug-cc-pVTZ basis set was used for the remaining systems. B-TCNE was not included because of computational cost. All values in eV.

| | $G_0W_0$@PBE | $G_{\mathrm{RS}}W_0$@PBE | $G_{\mathrm{RS}}W_{\mathrm{RS}}$@PBE | ev$GW$@PBE |
|---|---|---|---|---|
| acetaldehyde | 10.89 | 11.82 | 12.53 | 12.29 |
| acetone | 10.48 | 11.37 | 12.10 | 11.83 |
| formaldehyde | 11.43 | 12.27 | 12.90 | 12.72 |
| pyrazine | 9.05 | 9.72 | 10.30 | 10.15 |
| pyridazine | 8.54 | 9.36 | 9.98 | 9.78 |
| pyridine | 9.68 | 10.36 | 10.99 | 10.84 |
| pyrimidine | 9.41 | 10.12 | 10.74 | 10.56 |
| s-tetrazine | 7.66 | 8.39 | 9.01 | 8.83 |
| ethylene | 12.25 | 12.61 | 13.06 | 12.98 |
| butadiene | 9.53 | 9.89 | 10.32 | 10.22 |
| benzene | 10.18 | 10.58 | 11.00 | 10.91 |
| naphthalene | 7.92 | 8.29 | 8.68 | 8.60 |
| furan | 10.46 | 10.81 | 11.23 | 11.13 |
| hexatriene | 7.93 | 8.29 | 8.71 | 8.63 |
| water | 12.89 | 13.74 | 14.23 | 14.03 |

Table S2: Continued

| | $G_0W_0$@PBE | $G_{RS}W_0$@PBE | $G_{RS}W_{RS}$@PBE | ev$GW$@PBE |
|---|---|---|---|---|
| pNA | 7.27 | 7.86 | 8.39 | 8.27 |
| DMABN | 7.95 | 8.41 | 8.87 | 8.77 |

Table S3: Fundamental gaps of molecules in Truhlar-Gagliardi test set[S1] obtained from $G_0W_0$, $G_{RS}W_0$, $G_{RS}W_{RS}$ and ev$GW$ based on B3LYP. The aug-cc-pVDZ basis set was used for naphthalene, pNA and DMABN, and the aug-cc-pVTZ basis set was used for the remaining systems. B-TCNE was not included because of computational cost. All values in eV.

| | $G_0W_0$@B3LYP | $G_{RS}W_0$@B3LYP | $G_{RS}W_{RS}$@B3LYP | ev$GW$@B3LYP |
|---|---|---|---|---|
| acetaldehyde | 11.42 | 11.94 | 12.45 | 12.30 |
| acetone | 10.97 | 11.47 | 11.99 | 11.82 |
| formaldehyde | 11.76 | 12.26 | 12.71 | 12.56 |
| pyrazine | 9.51 | 9.90 | 10.33 | 10.21 |
| pyridazine | 9.04 | 9.58 | 10.01 | 9.81 |
| pyridine | 10.14 | 10.52 | 10.98 | 10.90 |
| pyrimidine | 9.86 | 10.28 | 10.74 | 10.61 |
| s-tetrazine | 8.17 | 8.60 | 9.07 | 8.87 |
| ethylene | 12.39 | 12.60 | 12.90 | 12.86 |
| butadiene | 9.83 | 10.04 | 10.34 | 10.29 |
| benzene | 10.45 | 10.70 | 10.99 | 10.91 |
| naphthalene | 8.21 | 8.44 | 8.71 | 8.61 |
| furan | 9.55 | 9.70 | 9.86 | 9.83 |
| hexatriene | 8.31 | 8.53 | 8.82 | 8.76 |
| water | 13.04 | 13.55 | 13.91 | 13.75 |
| pNA | 7.78 | 8.10 | 8.48 | 8.37 |
| DMABN | 8.27 | 8.54 | 8.87 | 8.76 |

Table S4: Fundamental gaps of molecules in Truhlar-Gagliardi test set[S1] obtained from $G_0W_0$, $G_{\mathrm{RS}}W_0$, $G_{\mathrm{RS}}W_{\mathrm{RS}}$ and ev$GW$ based on PBE0. The aug-cc-pVDZ basis set was used for naphthalene, pNA and DMABN, and the aug-cc-pVTZ basis set was used for the remaining systems. B-TCNE was not included because of computational cost. All values in eV.

| | $G_0W_0$@PBE0 | $G_{\mathrm{RS}}W_0$@PBE0 | $G_{\mathrm{RS}}W_{\mathrm{RS}}$@PBE0 | ev$GW$@PBE0 |
|---|---|---|---|---|
| acetaldehyde | 11.61 | 12.05 | 12.51 | 12.32 |
| acetone | 11.13 | 11.57 | 12.02 | 11.78 |
| formaldehyde | 11.94 | 12.37 | 12.77 | 12.61 |
| pyrazine | 9.67 | 10.00 | 10.38 | 10.25 |
| pyridazine | 9.23 | 9.69 | 10.08 | 9.85 |
| pyridine | 10.33 | 10.64 | 11.05 | 10.91 |
| pyrimidine | 10.04 | 10.40 | 10.81 | 10.63 |
| s-tetrazine | 8.32 | 8.69 | 9.11 | 8.92 |
| ethylene | 12.49 | 12.66 | 12.93 | 12.85 |
| butadiene | 9.94 | 10.12 | 10.38 | 10.29 |
| benzene | 10.55 | 10.75 | 11.00 | 10.93 |
| naphthalene | 8.30 | 8.51 | 8.74 | 8.63 |
| furan | 8.81 | 9.66 | 9.79 | 9.72 |
| hexatriene | 8.43 | 8.61 | 8.86 | 8.80 |
| water | 13.08 | 13.53 | 13.85 | 13.68 |
| pNA | 7.89 | 8.14 | 8.47 | 8.37 |
| DMABN | 8.39 | 8.62 | 8.91 | 8.79 |

# 2 Errors of using the linearized quasiparticle equation in $GW$

Table S5: Excitation energies of molecules in Truhlar-Gagliardi test set[S1] obtained from BSE/$G_{\mathrm{RS}}W_{\mathrm{RS}}$@B3LYP, where the quasiparticle equation in $G_{\mathrm{RS}}W_{\mathrm{RS}}$ is linearized and solved iteratively. The aug-cc-pVDZ basis set was used for naphthalene, pNA and DMABN, and the aug-cc-pVTZ basis set was used for the remaining systems. B-TCNE was not included because of computational cost. All values in eV.

| | state | linearized | iterative | difference |
|---|---|---|---|---|
| acetaldehyde | $^1A''$ | 4.22 | 4.20 | -0.02 |
| acetone | $^1A_2$ | 4.18 | 4.16 | -0.02 |

Table S5: Continued

| | state | linearized | iterative | difference |
|---|---|---|---|---|
| formaldehyde | $^1A_2$ | 3.81 | 3.79 | -0.02 |
| pyrazine | $^1B_{3u}$ | 4.05 | 4.04 | -0.02 |
| pyridazine | $^1B_1$ | 3.76 | 3.74 | -0.02 |
| pyridine | $^1B_1$ | 4.89 | 4.87 | -0.02 |
| pyrimidine | $^1B_1$ | 4.44 | 4.42 | -0.02 |
| s-tetrazine | $^1B_{3u}$ | 2.34 | 2.33 | -0.02 |
| ethylene | $^1B_{3u}$ | 6.77 | 6.77 | -0.01 |
| butadiene | $^1B_u$ | 5.89 | 5.88 | -0.01 |
| benzene | $^1B_{2u}$ | 5.19 | 5.18 | -0.01 |
| | $^3B_{1u}$ | 3.44 | 3.43 | -0.01 |
| naphthalene | $^1B_{3u}$ | 4.45 | 4.44 | -0.01 |
| | $^3B_{2u}$ | 2.64 | 2.63 | -0.01 |
| furan | $^1B_2$ | 5.70 | 5.69 | 0.00 |
| | $^3B_2$ | 3.34 | 3.33 | -0.01 |
| hexatriene | $^1B_u$ | 4.98 | 4.97 | -0.01 |
| | $^3B_u$ | 2.02 | 2.01 | -0.01 |
| water | Singlet | 6.94 | 6.92 | -0.02 |
| | Triplet | 6.15 | 6.13 | -0.02 |
| pNA | $^1A_1$ | 4.17 | 4.14 | -0.03 |
| DMABN | $^1A_1$ | 4.46 | 4.46 | 0.00 |

# 3 Fundamental gaps obtained from KS-DFT and KS-DFT with RS

Table S6: Fundamental gaps of molecules in Truhlar-Gagliardi test set[S1] obtained from PBE, PBE-RS, B3LYP and B3LYP-RS . The aug-cc-pVDZ basis set was used for naphthalene, pNA and DMABN, and the aug-cc-pVTZ basis set was used for the remaining systems. B-TCNE was not included because of computational cost. All values in eV.

| | PBE | RS-PBE | B3LYP | RS-B3LYP |
|---|---|---|---|---|
| acetaldehyde | 3.94 | 12.09 | 6.23 | 12.11 |
| acetone | 4.06 | 11.63 | 6.29 | 11.67 |

Table S6: Continued

| | PBE | RS-PBE | B3LYP | RS-B3LYP |
|---|---|---|---|---|
| formaldehyde | 3.59 | 12.69 | 5.92 | 12.68 |
| pyrazine | 3.25 | 9.50 | 5.30 | 9.56 |
| pyridazine | 2.78 | 10.23 | 4.89 | 10.27 |
| pyridine | 4.06 | 9.20 | 6.11 | 9.24 |
| pyrimidine | 3.61 | 10.03 | 5.68 | 10.08 |
| s-tetrazine | 1.52 | 10.74 | 3.67 | 10.83 |
| ethylene | 5.70 | 10.06 | 7.34 | 10.08 |
| butadiene | 4.01 | 8.44 | 5.50 | 8.51 |
| benzene | 5.15 | 8.91 | 6.62 | 8.94 |
| naphthalene | 3.52 | 7.38 | 4.84 | 7.48 |
| furan | 4.90 | 8.45 | 6.35 | 8.51 |
| hexatriene | 3.15 | 7.53 | 4.50 | 7.64 |
| water | 6.33 | 14.85 | 8.16 | 14.76 |
| pNA | 2.80 | 8.04 | 4.19 | 8.20 |
| DMABN | 3.55 | 7.48 | 4.95 | 7.62 |

# 4 Comparison between BSE/$G_{\mathrm{RS}}W_{\mathrm{RS}}$ and BSE-TDA/$G_{\mathrm{RS}}W_{\mathrm{RS}}$

Table S7: Excitation energies of systems in Truhlar-Gagliardi test set[S1] obtained from BSE/$G_{\mathrm{RS}}W_{\mathrm{RS}}$@PBE and BSE-TDA/$G_{\mathrm{RS}}W_{\mathrm{RS}}$@PBE. The aug-cc-pVDZ basis set was used for naphthalene, pNA and DMABN, and the aug-cc-pVTZ basis set was used for the remaining systems. B-TCNE was not included because of computational cost. All values in eV.

| molecule | state | BSE/$G_{\mathrm{RS}}W_{\mathrm{RS}}$ | BSE-TDA/$G_{\mathrm{RS}}W_{\mathrm{RS}}$ |
|---|---|---|---|
| acetaldehyde | 1A | 4.27 | 4.31 |
| acetone | 1A2 | 4.31 | 4.35 |
| formaldehyde | 1A2 | 3.90 | 3.95 |
| pyrazine | 1B3u | 4.01 | 4.07 |
| pyridazine | 1B1 | 3.73 | 3.81 |
| pyridine | 1B1 | 4.89 | 4.93 |
| pyrimidine | 1B1 | 4.42 | 4.45 |
| s-tetrazine | 1B3u | 2.29 | 2.38 |

Table S7: Continued

| molecule | state | BSE/$G_{\mathrm{RS}}W_{\mathrm{RS}}$ | BSE-TDA/$G_{\mathrm{RS}}W_{\mathrm{RS}}$ |
|---|---|---|---|
| ethylene | 1B1u | 6.65 | 6.67 |
| butadiene | 1Bu | 5.79 | 5.80 |
| benzene | 1B2u | 5.14 | 6.09 |
| | 3B1u | 3.35 | 5.94 |
| naphthalene | 1B3u | 4.43 | 4.46 |
| | 3B2u | 2.59 | 2.95 |
| furan | 1B2 | 5.58 | 5.59 |
| | 3B2 | 3.29 | 3.59 |
| hexatriene | 1Bu | 4.96 | 5.37 |
| | 3Bu | 1.86 | 2.33 |
| water | Singlet | 6.94 | 6.99 |
| | Triplet | 6.07 | 6.12 |
| pNA | 1A1 | 4.08 | 4.08 |
| DMABN | 1A1 | 4.48 | 4.30 |
| total MAE | | 0.45 | 0.45 |
| total ME | | -0.37 | -0.13 |
| singlet MAE | | 0.33 | 0.34 |
| singlet ME | | -0.37 | -0.09 |
| triplet MAE | | 0.86 | 0.82 |
| triplet ME | | -0.35 | -0.25 |

# 5 Results of Truhlar-Gagliardi test set

Table S8: Excitation energies of molecules in Truhlar-Gagliardi test set[S1] obtained from TDDFT based on HF, BLYP, PBE, B3LYP, PBE0 and PBEh(0.75). The aug-cc-pVDZ basis set was used for naphthalene, pNA and DMABN, and the aug-cc-pVTZ basis set was used for the remaining systems. B-TCNE was not included because of computational cost. Geometries were taken from Ref. S1. Reference values for pNA and DMABN were taken from Ref. S2 and for remaining molecules were taken from Ref. S3. All values in eV.

| | | | TDDFT | | | | | |
|---|---|---|---|---|---|---|---|---|
| | state | ref | HF | BLYP | PBE | B3LYP | PBE0 | PBEh |
| acetaldehyde | $^1A''$ | 4.31 | 4.86 | 4.19 | 4.17 | 4.31 | 4.32 | 4.66 |
| acetone | $^1A_2$ | 4.47 | 5.12 | 4.28 | 4.28 | 4.45 | 4.48 | 4.89 |
| formaldehyde | $^1A_2$ | 3.98 | 4.44 | 3.86 | 3.84 | 3.96 | 3.97 | 4.27 |
| pyrazine | $^1B_{3u}$ | 4.15 | 4.95 | 3.58 | 3.53 | 3.94 | 3.97 | 4.65 |
| pyridazine | $^1B_1$ | 3.83 | 4.74 | 3.12 | 3.09 | 3.55 | 3.62 | 4.42 |
| pyridine | $^1B_1$ | 4.95 | 5.99 | 4.36 | 4.33 | 4.78 | 4.85 | 5.65 |
| pyrimidine | $^1B_1$ | 4.44 | 5.76 | 3.83 | 3.79 | 4.29 | 4.35 | 5.30 |
| s-tetrazine | $^1B_{3u}$ | 2.47 | 3.28 | 1.86 | 1.80 | 2.22 | 2.25 | 2.94 |
| ethylene | $^1B_{3u}$ | 7.93 | 7.41 | 7.28 | 7.42 | 7.42 | 7.54 | 7.65 |
| butadiene | $^1B_u$ | 6.22 | 5.99 | 5.33 | 5.50 | 5.63 | 5.73 | 6.07 |
| benzene | $^1B_{2u}$ | 5.06 | 5.84 | 5.22 | 5.27 | 5.41 | 5.50 | 5.83 |
| | $^3B_{1u}$ | 4.16 | -2.08 | 4.08 | 4.05 | 3.85 | 3.65 | 2.12 |
| naphthalene | $^1B_{3u}$ | 4.00 | 4.80 | 4.09 | 4.13 | 4.40 | 4.50 | 4.89 |
| | $^3B_{2u}$ | 3.11 | -2.65 | 2.93 | 2.91 | 2.83 | 2.69 | 0.83 |
| furan | $^1B_2$ | 6.37 | 6.13 | 5.86 | 5.97 | 6.04 | 6.16 | 6.34 |
| | $^3B_2$ | 4.20 | -0.32 | 4.03 | 4.03 | 3.86 | 3.74 | 2.69 |
| hexatriene | $^1B_u$ | 5.37 | 5.18 | 4.48 | 4.52 | 4.70 | 4.78 | 5.18 |
| | $^3B_u$ | 2.73 | -2.46 | 2.43 | 2.39 | 2.26 | 2.07 | -0.78 |
| water | Singlet | 7.62 | 8.67 | 6.27 | 6.41 | 6.93 | 7.19 | 8.66 |
| | Triplet | 7.25 | 7.91 | 5.97 | 6.07 | 6.57 | 6.77 | 8.05 |
| pNA | $^1A_1$ | 4.39 | 5.12 | 3.52 | 3.56 | 3.96 | 4.12 | 4.94 |
| DMABN | $^1A_1$ | 4.86 | 5.27 | 4.33 | 4.35 | 4.67 | 4.76 | 5.25 |

Table S9: Excitation energies of molecules in Truhlar-Gagliardi test set[S1] obtained from BSE/$G_0W_0$ based on HF, BLYP, PBE, B3LYP, PBE0 and PBEh(0.75). The aug-cc-pVDZ basis set was used for naphthalene, pNA and DMABN, and the aug-cc-pVTZ basis set was used for the remaining systems. B-TCNE was not included because of computational cost. Geometries were taken from Ref. S1. Reference values for pNA and DMABN were taken from Ref. S2 and for remaining molecules were taken from Ref. S3. All values in eV.

| | | | BSE/$G_0W_0$ | | | | | |
|---|---|---|---|---|---|---|---|---|
| | state | ref | HF | BLYP | PBE | B3LYP | PBE0 | PBEh |
| acetaldehyde | $^1A''$ | 4.31 | 5.53 | 2.67 | 2.73 | 3.24 | 3.40 | 4.37 |
| acetone | $^1A_2$ | 4.47 | 5.97 | 2.74 | 2.81 | 3.25 | 3.39 | 4.60 |
| formaldehyde | $^1A_2$ | 3.98 | 5.11 | 2.46 | 2.51 | 2.91 | 2.94 | 3.91 |
| pyrazine | $^1B_{3u}$ | 4.15 | 5.35 | 2.77 | 2.81 | 3.26 | 3.39 | 4.28 |
| pyridazine | $^1B_1$ | 3.83 | 4.83 | 2.26 | 2.32 | 2.82 | 2.97 | 3.96 |
| pyridine | $^1B_1$ | 4.95 | 6.50 | 3.56 | 3.62 | 4.09 | 4.24 | 5.20 |
| pyrimidine | $^1B_1$ | 4.44 | 5.63 | 3.09 | 3.14 | 3.60 | 3.74 | 4.64 |
| s-tetrazine | $^1B_{3u}$ | 2.47 | 2.94 | 0.92 | 0.95 | 1.46 | 1.58 | 2.49 |
| ethylene | $^1B_{3u}$ | 7.93 | 7.67 | 6.65 | 6.69 | 6.93 | 7.00 | 7.41 |
| butadiene | $^1B_u$ | 6.22 | 6.74 | 5.02 | 5.04 | 5.34 | 5.42 | 5.86 |
| benzene | $^1B_{2u}$ | 5.06 | 6.20 | 4.33 | 4.35 | 4.67 | 4.75 | 5.32 |
| | $^3B_{1u}$ | 4.16 | 4.77 | 2.45 | 2.47 | 2.89 | 2.98 | 3.72 |
| naphthalene | $^1B_{3u}$ | 4.00 | 4.93 | 3.71 | 3.73 | 4.03 | 4.11 | 4.60 |
| | $^3B_{2u}$ | 3.11 | 3.34 | 1.72 | 1.74 | 2.14 | 2.23 | 2.83 |
| furan | $^1B_2$ | 6.37 | 6.90 | 5.22 | 5.21 | 5.53 | 5.57 | 6.03 |
| | $^3B_2$ | 4.20 | 4.63 | 2.49 | 2.48 | 2.84 | 2.90 | 3.59 |
| hexatriene | $^1B_u$ | 5.37 | 5.65 | 4.09 | 4.11 | 4.44 | 4.52 | 5.00 |
| | $^3B_u$ | 2.73 | 3.41 | 0.68 | 0.69 | 1.40 | 1.52 | 2.40 |
| water | Singlet | 7.62 | 8.13 | 5.58 | 5.64 | 6.08 | 6.25 | 7.34 |
| | Triplet | 7.25 | 7.66 | 4.71 | 4.77 | 5.29 | 5.48 | 6.77 |
| pNA | $^1A_1$ | 4.39 | 4.69 | 3.24 | 3.23 | 3.71 | 3.79 | 4.39 |
| DMABN | $^1A_1$ | 4.86 | 5.44 | 4.03 | 4.08 | 4.35 | 4.44 | 4.86 |

Table S10: Excitation energies of molecules in Truhlar-Gagliardi test set[S1] obtained from BSE/$G_{\mathrm{RS}}W_0$ based on HF, BLYP, PBE, B3LYP, PBE0 and PBEh(0.75). The aug-cc-pVDZ basis set was used for naphthalene, pNA and DMABN, and the aug-cc-pVTZ basis set was used for the remaining systems. B-TCNE was not included because of computational cost. Geometries were taken from Ref. S1. Reference values for pNA and DMABN were taken from Ref. S2 and for remaining molecules were taken from Ref. S3. All values in eV.

| | | | BSE/$G_{\mathrm{RS}}W_0$ | | | | | |
|---|---|---|---|---|---|---|---|---|
| | state | ref | HF | BLYP | PBE | B3LYP | PBE0 | PBEh |
| acetaldehyde | $^1A''$ | 4.31 | 5.53 | 3.55 | 3.60 | 3.73 | 3.83 | 4.41 |
| acetone | $^1A_2$ | 4.47 | 5.97 | 3.58 | 3.64 | 3.72 | 3.79 | 4.64 |
| formaldehyde | $^1A_2$ | 3.98 | 5.11 | 3.25 | 3.31 | 3.39 | 3.46 | 3.94 |
| pyrazine | $^1B_{3u}$ | 4.15 | 5.35 | 3.45 | 3.45 | 3.63 | 3.70 | 4.34 |
| pyridazine | $^1B_1$ | 3.83 | 4.83 | 3.09 | 3.12 | 3.34 | 3.43 | 3.99 |
| pyridine | $^1B_1$ | 4.95 | 6.50 | 4.23 | 4.27 | 4.45 | 4.54 | 5.25 |
| pyrimidine | $^1B_1$ | 4.44 | 5.63 | 3.79 | 3.82 | 4.00 | 4.09 | 4.69 |
| s-tetrazine | $^1B_{3u}$ | 2.47 | 2.94 | 1.68 | 1.69 | 1.89 | 1.94 | 2.55 |
| ethylene | $^1B_{3u}$ | 7.93 | 7.67 | 7.03 | 7.04 | 7.14 | 7.16 | 7.41 |
| butadiene | $^1B_u$ | 6.22 | 6.74 | 5.43 | 5.44 | 5.57 | 5.61 | 5.87 |
| benzene | $^1B_{2u}$ | 5.06 | 6.20 | 4.74 | 4.74 | 4.91 | 4.94 | 5.33 |
| | $^3B_{1u}$ | 4.16 | 4.77 | 2.92 | 2.91 | 3.14 | 3.19 | 3.73 |
| naphthalene | $^1B_{3u}$ | 4.00 | 4.93 | 4.11 | 4.11 | 4.28 | 4.31 | 4.62 |
| | $^3B_{2u}$ | 3.11 | 3.34 | 2.17 | 2.18 | 2.40 | 2.45 | 2.85 |
| furan | $^1B_2$ | 6.37 | 6.90 | 5.60 | 5.58 | 5.74 | 5.75 | 6.02 |
| | $^3B_2$ | 4.20 | 4.63 | 2.87 | 2.86 | 3.05 | 3.08 | 3.58 |
| hexatriene | $^1B_u$ | 5.37 | 5.65 | 4.52 | 4.51 | 4.67 | 4.71 | 5.01 |
| | $^3B_u$ | 2.73 | 3.41 | 1.36 | 1.33 | 1.67 | 1.74 | 2.41 |
| water | Singlet | 7.62 | 8.13 | 6.44 | 6.47 | 6.59 | 6.69 | 7.37 |
| | Triplet | 7.25 | 7.66 | 5.57 | 5.60 | 5.80 | 5.92 | 6.80 |
| pNA | $^1A_1$ | 4.39 | 4.69 | 3.88 | 3.86 | 4.04 | 4.06 | 4.41 |
| DMABN | $^1A_1$ | 4.86 | 5.44 | 4.52 | 4.55 | 4.62 | 4.68 | 4.88 |

Table S11: Excitation energies of molecules in Truhlar-Gagliardi test set[S1] obtained from BSE/$G_{\mathrm{RS}}W_{\mathrm{RS}}$ based on HF, BLYP, PBE, B3LYP, PBE0 and PBEh(0.75). The aug-cc-pVDZ basis set was used for naphthalene, pNA and DMABN, and the aug-cc-pVTZ basis set was used for the remaining systems. B-TCNE was not included because of computational cost. Geometries were taken from Ref. S1. Reference values for pNA and DMABN were taken from Ref. S2 and for remaining molecules were taken from Ref. S3. All values in eV.

| | | | BSE/$G_{\mathrm{RS}}W_{\mathrm{RS}}$ | | | | | |
|---|---|---|---|---|---|---|---|---|
| | state | ref | HF | BLYP | PBE | B3LYP | PBE0 | PBEh |
| acetaldehyde | $^1A''$ | 4.31 | 5.53 | 4.23 | 4.27 | 4.22 | 4.25 | 4.48 |
| acetone | $^1A_2$ | 4.47 | 5.97 | 4.27 | 4.31 | 4.18 | 4.20 | 4.71 |
| formaldehyde | $^1A_2$ | 3.98 | 5.11 | 3.86 | 3.90 | 3.81 | 3.84 | 4.00 |
| pyrazine | $^1B_{3u}$ | 4.15 | 5.35 | 4.02 | 4.01 | 4.05 | 4.08 | 4.39 |
| pyridazine | $^1B_1$ | 3.83 | 4.83 | 3.71 | 3.73 | 3.76 | 3.80 | 4.04 |
| pyridine | $^1B_1$ | 4.95 | 6.50 | 4.86 | 4.89 | 4.89 | 4.93 | 5.30 |
| pyrimidine | $^1B_1$ | 4.44 | 5.63 | 4.41 | 4.42 | 4.44 | 4.48 | 4.75 |
| s-tetrazine | $^1B_{3u}$ | 2.47 | 2.94 | 2.29 | 2.29 | 2.34 | 2.35 | 2.63 |
| ethylene | $^1B_{3u}$ | 7.93 | 7.67 | 7.53 | 7.54 | 7.46 | 7.45 | 7.44 |
| butadiene | $^1B_u$ | 6.22 | 6.74 | 5.90 | 5.90 | 5.89 | 5.89 | 5.90 |
| benzene | $^1B_{2u}$ | 5.06 | 6.20 | 5.16 | 5.14 | 5.19 | 5.18 | 5.36 |
| | $^3B_{1u}$ | 4.16 | 4.77 | 3.36 | 3.35 | 3.44 | 3.44 | 3.77 |
| naphthalene | $^1B_{3u}$ | 4.00 | 4.93 | 4.51 | 4.50 | 4.55 | 4.55 | 4.65 |
| | $^3B_{2u}$ | 3.11 | 3.34 | 2.60 | 2.60 | 2.68 | 2.69 | 2.88 |
| furan | $^1B_2$ | 6.37 | 6.90 | 6.05 | 6.02 | 6.04 | 6.01 | 6.05 |
| | $^3B_2$ | 4.20 | 4.63 | 3.31 | 3.29 | 3.34 | 3.32 | 3.61 |
| hexatriene | $^1B_u$ | 5.37 | 5.65 | 4.97 | 4.96 | 4.98 | 4.99 | 5.05 |
| | $^3B_u$ | 2.73 | 3.41 | 1.88 | 1.86 | 2.02 | 2.04 | 2.44 |
| water | Singlet | 7.62 | 8.13 | 6.92 | 6.94 | 6.94 | 7.00 | 7.43 |
| | Triplet | 7.25 | 7.66 | 6.06 | 6.07 | 6.15 | 6.23 | 6.86 |
| pNA | $^1A_1$ | 4.39 | 4.69 | 4.45 | 4.41 | 4.43 | 4.39 | 4.47 |
| DMABN | $^1A_1$ | 4.86 | 5.44 | 4.97 | 5.03 | 4.96 | 4.97 | 4.93 |

Table S12: Excitation energies of molecules in Truhlar-Gagliardi test set[S1] obtained from BSE/ev$GW$ based on HF, BLYP, PBE, B3LYP, PBE0 and PBEh(0.75). The aug-cc-pVDZ basis set was used for naphthalene, pNA and DMABN, and the aug-cc-pVTZ basis set was used for the remaining systems. B-TCNE was not included because of computational cost. Geometries were taken from Ref. S1. Reference values for pNA and DMABN were taken from Ref. S2 and for remaining molecules were taken from Ref. S3. All values in eV.

| | | | BSE/ev$GW$ | | | | | |
|---|---|---|---|---|---|---|---|---|
| | state | ref | HF | BLYP | PBE | B3LYP | PBE0 | PBEh |
| acetaldehyde | $^1A''$ | 4.31 | 5.46 | 4.02 | 4.04 | 4.07 | 4.08 | 4.34 |
| acetone | $^1A_2$ | 4.47 | 5.90 | 4.01 | 4.06 | 4.03 | 3.98 | 4.55 |
| formaldehyde | $^1A_2$ | 3.98 | 5.04 | 3.68 | 3.73 | 3.67 | 3.69 | 3.90 |
| pyrazine | $^1B_{3u}$ | 4.15 | 5.25 | 3.86 | 3.87 | 3.94 | 3.95 | 4.20 |
| pyridazine | $^1B_1$ | 3.83 | 4.69 | 3.52 | 3.54 | 3.57 | 3.58 | 3.88 |
| pyridine | $^1B_1$ | 4.95 | 6.43 | 4.72 | 4.75 | 4.81 | 4.80 | 5.13 |
| pyrimidine | $^1B_1$ | 4.44 | 5.53 | 4.24 | 4.25 | 4.31 | 4.31 | 4.57 |
| s-tetrazine | $^1B_{3u}$ | 2.47 | 2.75 | 2.12 | 2.12 | 2.15 | 2.17 | 2.41 |
| ethylene | $^1B_{3u}$ | 7.93 | 8.23 | 7.46 | 7.50 | 7.43 | 7.41 | 7.43 |
| butadiene | $^1B_u$ | 6.22 | 6.74 | 5.80 | 5.75 | 5.83 | 5.79 | 5.86 |
| benzene | $^1B_{2u}$ | 5.06 | 6.15 | 5.04 | 5.06 | 6.13 | 6.12 | 5.29 |
| | $^3B_{1u}$ | 4.16 | 4.72 | 3.24 | 3.26 | 6.00 | 5.99 | 3.69 |
| naphthalene | $^1B_{3u}$ | 4.00 | 5.32 | 4.42 | 4.46 | 4.44 | 4.44 | 4.54 |
| | $^3B_{2u}$ | 3.11 | 3.42 | 2.52 | 2.49 | 2.58 | 2.59 | 2.75 |
| furan | $^1B_2$ | 6.37 | 6.89 | 5.93 | 5.91 | 5.98 | 5.89 | 6.01 |
| | $^3B_2$ | 4.20 | 4.63 | 3.20 | 3.18 | 3.29 | 3.21 | 3.58 |
| hexatriene | $^1B_u$ | 5.37 | 5.63 | 4.88 | 4.88 | 4.92 | 4.92 | 4.99 |
| | $^3B_u$ | 2.73 | 3.40 | 1.79 | 1.77 | 1.96 | 1.98 | 2.39 |
| water | Singlet | 7.62 | 8.03 | 6.73 | 6.75 | 6.78 | 6.84 | 7.32 |
| | Triplet | 7.25 | 7.57 | 5.87 | 5.88 | 5.99 | 6.07 | 6.74 |
| pNA | $^1A_1$ | 4.39 | 4.60 | 4.32 | 4.28 | 4.31 | 4.28 | 4.32 |
| DMABN | $^1A_1$ | 4.86 | 5.83 | 4.89 | 4.92 | 4.84 | 4.85 | 4.80 |

# 6 Results of Stein CT test set

Table S13: Excitation energies of charge transfer systems in Stein CT test set[S4] obtained from TDDFT with HF, BLYP, PBE, B3LYP, PBE0 and PBEh(0.75). Gas phase results were taken as the reference.[S4] The cc-pVDZ basis set was used. All values in eV.

| | | TDDFT | | | | | |
|---|---|---|---|---|---|---|---|
| | ref | HF | BLYP | PBE | B3LYP | PBE0 | PBEh |
| anthracene | 2.05 | 2.83 | 1.46 | 1.46 | 1.55 | 1.59 | 2.24 |
| 9-cyano | 2.33 | 3.19 | 0.72 | 0.72 | 0.82 | 0.91 | 2.32 |
| 9-cholo | 2.06 | 2.92 | 1.23 | 1.23 | 1.32 | 1.36 | 2.22 |
| 9-carbo-methoxy | 2.16 | 3.00 | 1.13 | 1.12 | 1.23 | 1.28 | 2.26 |
| 9-methyl | 1.87 | 2.65 | 1.34 | 1.34 | 1.41 | 1.44 | 2.06 |
| 9,10-dimethyl | 1.76 | 2.59 | 1.60 | 1.60 | 1.67 | 1.70 | 2.14 |
| 9-formyl | 2.22 | 3.07 | 0.87 | 0.79 | 1.27 | 1.33 | 2.34 |
| 9-formyl, 10-chloro | 2.28 | 3.17 | 0.85 | 0.78 | 1.22 | 1.30 | 2.41 |
| benzene | 3.91 | 4.64 | 1.42 | 1.42 | 1.98 | 2.14 | 3.73 |
| toluene | 3.68 | 4.32 | 1.38 | 1.37 | 1.82 | 1.95 | 3.43 |
| o-xylene | 3.47 | 4.08 | 1.07 | 1.06 | 1.54 | 1.68 | 3.18 |
| naphthalene | 2.92 | 3.56 | 0.34 | 0.36 | 0.90 | 1.07 | 2.66 |

Table S14: Excitation energies of charge transfer systems in Stein CT test set[S4] obtained from BSE/$G_0W_0$ with HF, BLYP, PBE, B3LYP, PBE0 and PBEh(0.75). Gas phase results were taken as the reference.[S4] The cc-pVDZ basis set was used. All values in eV.

| | | BSE/$G_0W_0$ | | | | | |
|---|---|---|---|---|---|---|---|
| | ref | HF | BLYP | PBE | B3LYP | PBE0 | PBEh |
| anthracene | 2.05 | 2.02 | 0.95 | 0.90 | 1.41 | 1.47 | 2.26 |
| 9-cyano | 2.33 | 2.39 | 1.33 | 1.34 | 1.34 | 1.58 | 2.41 |
| 9-cholo | 2.06 | 2.09 | 0.69 | 0.65 | 1.30 | 1.40 | 2.23 |
| 9-carbo-methoxy | 2.16 | 2.17 | 0.61 | 0.55 | 1.30 | 1.41 | 2.25 |
| 9-methyl | 1.87 | 1.86 | 0.72 | 0.67 | 1.22 | 1.29 | 2.09 |
| 9,10-dimethyl | 1.76 | 1.83 | 1.01 | 0.97 | 1.39 | 1.43 | 2.16 |
| 9-formyl | 2.22 | 2.24 | 0.72 | 0.69 | 1.43 | 1.55 | 2.35 |
| 9-formyl, 10-chloro | 2.28 | 2.33 | 0.68 | 0.66 | 1.47 | 1.61 | 2.39 |
| benzene | 3.91 | 3.74 | 2.72 | 2.69 | 3.22 | 3.26 | 3.91 |
| toluene | 3.68 | 3.43 | 2.18 | 2.15 | 2.86 | 2.91 | 3.61 |
| o-xylene | 3.47 | 3.15 | 1.82 | 1.78 | 2.52 | 2.59 | 3.29 |

Table S14: Continued

| | | BSE/$G_0W_0$ | | | | | |
|---|---|---|---|---|---|---|---|
| | ref | HF | BLYP | PBE | B3LYP | PBE0 | PBEh |
| naphthalene | 2.92 | 2.74 | 1.90 | 1.91 | 2.33 | 2.35 | 2.86 |

Table S15: Excitation energies of charge transfer systems in Stein CT test set[S4] obtained from BSE/$G_{\mathrm{RS}}W_0$ with HF, BLYP, PBE, B3LYP, PBE0 and PBEh(0.75). Gas phase results were taken as the reference.[S4] The cc-pVDZ basis set was used. All values in eV.

| | | BSE/$G_{\mathrm{RS}}W_0$ | | | | | |
|---|---|---|---|---|---|---|---|
| | ref | HF | BLYP | PBE | B3LYP | PBE0 | PBEh |
| anthracene | 2.05 | 2.02 | 1.87 | 1.84 | 1.89 | 1.87 | 1.94 |
| 9-cyano | 2.33 | 2.39 | 1.89 | 1.86 | 2.00 | 2.04 | 2.29 |
| 9-cholo | 2.06 | 2.09 | 1.82 | 1.79 | 1.85 | 1.85 | 2.00 |
| 9-carbo-methoxy | 2.16 | 2.17 | 1.84 | 1.81 | 1.87 | 1.86 | 2.07 |
| 9-methyl | 1.87 | 1.86 | 1.72 | 1.69 | 1.73 | 1.71 | 1.78 |
| 9,10-dimethyl | 1.76 | 1.83 | 1.80 | 1.77 | 1.82 | 1.80 | 1.80 |
| 9-formyl | 2.22 | 2.24 | 1.92 | 1.98 | 1.97 | 1.98 | 2.15 |
| 9-formyl, 10-chloro | 2.28 | 2.33 | 1.95 | 1.96 | 2.01 | 2.03 | 2.24 |
| benzene | 3.91 | 3.74 | 3.43 | 3.37 | 3.54 | 3.52 | 3.63 |
| toluene | 3.68 | 3.43 | 3.10 | 3.05 | 3.22 | 3.20 | 3.32 |
| o-xylene | 3.47 | 3.15 | 2.75 | 2.70 | 2.88 | 2.87 | 3.03 |
| naphthalene | 2.92 | 2.74 | 2.44 | 2.40 | 2.52 | 2.52 | 2.65 |

Table S16: Excitation energies of charge transfer systems in Stein CT test set[S4] obtained from BSE/$G_{\mathrm{RS}}W_{\mathrm{RS}}$ with HF, BLYP, PBE, B3LYP, PBE0 and PBEh(0.75). Gas phase results were taken as the reference.[S4] The cc-pVDZ basis set was used. All values in eV.

| | | BSE/$G_{\mathrm{RS}}W_{\mathrm{RS}}$ | | | | | |
|---|---|---|---|---|---|---|---|
| | ref | HF | BLYP | PBE | B3LYP | PBE0 | PBEh |
| anthracene | 2.05 | 2.02 | 2.33 | 2.30 | 2.26 | 2.33 | 2.03 |
| 9-cyano | 2.33 | 2.39 | 2.39 | 2.36 | 2.41 | 2.39 | 2.37 |
| 9-cholo | 2.06 | 2.09 | 2.29 | 2.26 | 2.23 | 2.29 | 2.09 |
| 9-carbo-methoxy | 2.16 | 2.17 | 2.32 | 2.29 | 2.25 | 2.32 | 2.15 |
| 9-methyl | 1.87 | 1.86 | 2.17 | 2.14 | 2.09 | 2.17 | 1.87 |

Table S16: Continued

| | | BSE/$G_{RS}W_{RS}$ | | | | | |
|---|---|---|---|---|---|---|---|
| | ref | HF | BLYP | PBE | B3LYP | PBE0 | PBEh |
| 9,10-dimethyl | 1.76 | 1.83 | 2.23 | 2.20 | 2.16 | 2.23 | 1.89 |
| 9-formyl | 2.22 | 2.24 | 2.40 | 2.50 | 2.35 | 2.40 | 2.24 |
| 9-formyl, 10-chloro | 2.28 | 2.33 | 2.43 | 2.45 | 2.39 | 2.43 | 2.33 |
| benzene | 3.91 | 3.74 | 3.95 | 3.89 | 3.91 | 3.95 | 3.71 |
| toluene | 3.68 | 3.43 | 3.65 | 3.60 | 3.61 | 3.65 | 3.40 |
| o-xylene | 3.47 | 3.15 | 3.31 | 3.25 | 3.29 | 3.31 | 3.12 |
| naphthalene | 2.92 | 2.74 | 2.90 | 2.85 | 2.86 | 2.90 | 2.72 |

# 7 Results of Rydberg excitations

Table S17: Mean absolute errors (MAEs) and mean signed errors (MSEs) of $B^+$, Be and Mg obtained from TDDFT, BSE/$G_0W_0$, BSE/$G_{RS}W_0$, BSE/$G_{RS}W_{RS}$ and BSE/ev$GW$ with HF, BLYP, PBE, B3LYP and PBE0. All values in eV. References were taken from Ref. S5. The aug-cc-pVQZ basis set was used.

| | HF | | BLYP | | PBE | | B3LYP | | PBE0 | |
|---|---|---|---|---|---|---|---|---|---|---|
| | MAE | MSE | MAE | MSE | MAE | MSE | MAE | MSE | MAE | MSE |
| TDDFT | 0.92 | -0.92 | 1.17 | -1.17 | 1.03 | -1.03 | 0.89 | -0.89 | 0.80 | -0.80 |
| BSE/$G_0W_0$ | 0.16 | -0.11 | 1.00 | -1.00 | 0.97 | -0.97 | 0.73 | -0.73 | 0.64 | -0.64 |
| BSE/$G_{RS}W_0$ | 0.16 | -0.11 | 0.84 | -0.84 | 0.82 | -0.82 | 0.69 | -0.69 | 0.62 | -0.62 |
| BSE/$G_{RS}W_{RS}$ | 0.16 | -0.11 | 0.69 | -0.69 | 0.69 | -0.69 | 0.63 | -0.63 | 0.57 | -0.57 |
| BSE/ev$GW$ | 0.15 | -0.07 | 0.65 | -0.65 | 0.65 | -0.65 | 0.59 | -0.59 | 0.54 | -0.54 |

Table S18: Rydberg excitation energies of Be, $B^+$ and Mg obtained from TDDFT with HF, BLYP, PBE, B3LYP and PBE0. Reference values were from Ref. S5. The aug-cc-pVQZ basis set was used. All values in eV.

| | | | TDDFT | | | | |
|---|---|---|---|---|---|---|---|
| | state | ref | HF | BLYP | PBE | B3LYP | PBE0 |
| Be | triplet 2s→3s | 6.46 | 5.49 | 5.37 | 5.47 | 5.65 | 5.70 |
| | singlet 2s→3s | 6.78 | 6.13 | 5.55 | 5.75 | 5.88 | 6.03 |
| $B^+$ | triplet 2s→3s | 16.09 | 14.76 | 14.68 | 14.78 | 14.96 | 15.02 |
| | singlet 2s→3s | 17.06 | 15.82 | 15.26 | 15.45 | 15.58 | 15.74 |

Table S18: Continued

| | state | ref | TDDFT | | | | |
|---|---|---|---|---|---|---|---|
| | | | HF | BLYP | PBE | B3LYP | PBE0 |
| Mg | triplet 3s→4s | 5.11 | 4.32 | 4.45 | 4.52 | 4.67 | 4.68 |
| | singlet 3s→4s | 5.39 | 4.84 | 4.57 | 4.73 | 4.83 | 4.93 |

Table S19: Rydberg excitation energies of Be, $B^+$ and Mg obtained from BSE/$G_0W_0$ with HF, BLYP, PBE, B3LYP and PBE0. Reference values were from Ref. S5. The aug-cc-pVQZ basis set was used. All values in eV.

| | state | ref | BSE/$G_0W_0$ | | | | |
|---|---|---|---|---|---|---|---|
| | | | HF | BLYP | PBE | B3LYP | PBE0 |
| Be | triplet 2s→3s | 6.46 | 6.24 | | | 5.50 | 5.62 |
| | singlet 2s→3s | 6.78 | 6.83 | 6.27 | 6.30 | 6.47 | 6.52 |
| $B^+$ | triplet 2s→3s | 16.09 | 15.83 | 14.29 | 14.30 | 14.82 | 14.96 |
| | singlet 2s→3s | 17.06 | 16.82 | 15.83 | 15.85 | 16.31 | 16.36 |
| Mg | triplet 3s→4s | 5.11 | 5.01 | 4.09 | 4.12 | 4.32 | 4.42 |
| | singlet 3s→4s | 5.39 | 5.49 | 4.96 | 5.00 | 5.11 | 5.17 |

Table S20: Rydberg excitation energies of Be, $B^+$ and Mg obtained from BSE/$G_{\mathrm{RS}}W_0$ with HF, BLYP, PBE, B3LYP and PBE0. Reference values were from Ref. S5. The aug-cc-pVQZ basis set was used. All values in eV.

| | state | ref | BSE/$G_{\mathrm{RS}}W_0$ | | | | |
|---|---|---|---|---|---|---|---|
| | | | HF | BLYP | PBE | B3LYP | PBE0 |
| Be | triplet 2s→3s | 6.46 | 6.24 | 5.40 | 5.39 | 5.59 | 5.68 |
| | singlet 2s→3s | 6.78 | 6.83 | 6.46 | 6.46 | 6.54 | 6.57 |
| $B^+$ | triplet 2s→3s | 16.09 | 15.83 | 14.60 | 14.62 | 14.79 | 14.92 |
| | singlet 2s→3s | 17.06 | 16.82 | 16.17 | 16.17 | 16.28 | 16.32 |
| Mg | triplet 3s→4s | 5.11 | 5.01 | 4.12 | 4.23 | 4.37 | 4.47 |
| | singlet 3s→4s | 5.39 | 5.49 | 5.10 | 5.12 | 5.16 | 5.21 |

Table S21: Rydberg excitation energies of Be, $B^+$ and Mg obtained from BSE/$G_{RS}W_{RS}$ with HF, BLYP, PBE, B3LYP and PBE0. Reference values were from Ref. S5. The aug-cc-pVQZ basis set was used. All values in eV.

| | | | BSE/$G_{RS}W_{RS}$ | | | | |
|---|---|---|---|---|---|---|---|
| | state | ref | HF | BLYP | PBE | B3LYP | PBE0 |
| Be | triplet 2s→3s | 6.46 | 6.24 | 5.57 | 5.57 | 5.68 | 5.75 |
| | singlet 2s→3s | 6.78 | 6.83 | 6.61 | 6.60 | 6.62 | 6.64 |
| $B^+$ | triplet 2s→3s | 16.09 | 15.83 | 14.73 | 14.75 | 14.86 | 14.96 |
| | singlet 2s→3s | 17.06 | 16.82 | 16.32 | 16.32 | 16.35 | 16.36 |
| Mg | triplet 3s→4s | 5.11 | 5.01 | 4.34 | 4.34 | 4.43 | 4.50 |
| | singlet 3s→4s | 5.39 | 5.49 | 5.20 | 5.20 | 5.20 | 5.24 |

Table S22: Rydberg excitation energies of Be, $B^+$ and Mg obtained from BSE/ev$GW$ with HF, BLYP, PBE, B3LYP and PBE0. Reference values were from Ref. S5. The aug-cc-pVQZ basis set was used. All values in eV.

| | | | BSE/BSE/ev$GW$ | | | | |
|---|---|---|---|---|---|---|---|
| | state | ref | HF | BLYP | PBE | B3LYP | PBE0 |
| Be | triplet 2s→3s | 6.46 | 6.29 | 5.60 | 5.59 | 5.70 | 5.77 |
| | singlet 2s→3s | 6.78 | 6.87 | 6.64 | 6.62 | 6.65 | 6.66 |
| $B^+$ | triplet 2s→3s | 16.09 | 15.87 | 14.78 | 14.81 | 14.92 | 15.0 |
| | singlet 2s→3s | 17.06 | 16.86 | 16.38 | 16.38 | 16.40 | 16.4 |
| Mg | triplet 3s→4s | 5.11 | 5.06 | 4.38 | 4.37 | 4.46 | 4.54 |
| | singlet 3s→4s | 5.39 | 5.53 | 5.23 | 5.24 | 5.24 | 5.27 |

# References


(S1) Hoyer, C. E.; Ghosh, S.; Truhlar, D. G.; Gagliardi, L. Multiconfiguration Pair-Density Functional Theory Is as Accurate as CASPT2 for Electronic Excitation. *J. Phys. Chem. Lett.* **2016**, *7*, 586–591.

(S2) Gui, X.; Holzer, C.; Klopper, W. Accuracy Assessment of GW Starting Points for Calculating Molecular Excitation Energies Using the Bethe–Salpeter Formalism. *J. Chem. Theory Comput.* **2018**, *14*, 2127–2136.

(S3) Véril, M.; Scemama, A.; Caffarel, M.; Lipparini, F.; Boggio-Pasqua, M.; Jacquemin, D.; Loos, P.-F. QUESTDB:

A Database of Highly Accurate Excitation Energies for the Electronic Structure Community. *WIREs Comput. Mol. Sci.* **2021**, *11*, e1517.

(S4) Stein, T.; Kronik, L.; Baer, R. Reliable Prediction of Charge Transfer Excitations in Molecular Complexes Using Time-Dependent Density Functional Theory. *J. Am. Chem. Soc.* **2009**, *131*, 2818–2820.

(S5) Xu, X.; Yang, K. R.; Truhlar, D. G. Testing Noncollinear Spin-Flip, Collinear Spin-Flip, and Conventional Time-Dependent Density Functional Theory for Predicting Electronic Excitation Energies of Closed-Shell Atoms. *J. Chem. Theory Comput.* **2014**, *10*, 2070–2084.
